# Supplementary material for: Gaussian Process Priors for View-Aware Inference
Source: arXiv:1912.03249 source file (2021-03-03)
Supplement: Supplementary file 3 [file sep_cov.tex]

% This file was created by tikzplotlib v0.9.1.
\begin{tikzpicture}

\begin{axis}[
hide x axis,
hide y axis,
tick align=outside,
tick pos=left,
x grid style={white!69.0196078431373!black},
xmin=-0.5, xmax=59.5,
xtick style={color=black},
y dir=reverse,
y grid style={white!69.0196078431373!black},
ymin=-0.5, ymax=59.5,
ytick style={color=black}
]
\addplot graphics [includegraphics cmd=\pgfimage,xmin=-0.5, xmax=59.5, ymin=59.5, ymax=-0.5] {sep_cov-000.png};
\end{axis}

\end{tikzpicture}
